# Supplementary material for: Non-destructive optical read-out and manipulation of circular Rydberg atoms
Source: arXiv:2509.24691 ancillary file (2025-09-29)
Supplement: Supplementary file 1 [file Machu2025_Supplementary_Material.pdf]

# SUPPLEMENTARY INFORMATION: Non-destructive optical read-out and manipulation of circular Rydberg atoms

Y. Machu,<sup>1</sup> A. Durán-Hernández,<sup>1</sup> G. Creutzer,<sup>1</sup> A. A. Young,<sup>1</sup> J. M. Raimond,<sup>1</sup> M. Brune,<sup>1</sup> and C. Sayrin<sup>1,2,\*</sup>

<sup>1</sup>*Laboratoire Kastler Brossel, Collège de France, CNRS, ENS-Université PSL,  
Sorbonne Université, 11 place Marcelin Berthelot, F-75231 Paris, France*

<sup>2</sup>*Institut Universitaire de France, 1 rue Descartes, 75231 Paris Cedex 05, France*

(Dated: September 28, 2025)

In this Supplementary Information, we describe in appendix A the experimental setup, the arrays of trapping sites that we use in the experiment and the main steps of an experimental sequence. In appendix B, we discuss the choice of levels to achieve a Förster resonance. Finally, in appendix C, we describe the experimental imperfection model and its fit to the data.

## Appendix A: Experimental procedures

### 1. Experimental setup

The experimental setup is described in details in [1] and is sketched in Fig. A.1. The atoms are trapped inside a hollow sapphire cube, which is held under ultra high vacuum. The cube supports electrodes to dynamically control the DC or radio-frequency electric fields and two tightly-focusing lenses,  $L_1$  and  $L_2$ , used for the generation of the trapping sites (see Sec. A 2). The Rydberg-excitation laser beams and an additional laser beam, used to optically pump and push-out ground-state atoms, enter the cube along the  $x$  axis (see Fig. A.1 for axes definition). All trapping laser beams enter along the  $y$  axis and are focused by lens  $L_1$  onto the atoms. This same lens collects the fluorescence photons emitted by the trapped atoms, and directs them towards an EMCCD camera.

### 2. Generation of the trapping sites

We prepare three different arrays of trapping sites by holography, using three liquid-crystal spatial light modulators [SLM, Hamamatsu LCOS X10468 (SLM1 and 3) and X15213 (SLM2)]. An SLM imprints a digitally-controllable phase mask on the impinging collimated Gaussian beam. We program a phase mask so that its diffraction pattern, obtained in the focal plane of the tightly-focusing lens  $L_1$  (focal length  $f = 16.32$  mm, numerical aperture  $NA = 0.27$ ), corresponds to the desired array of trapping sites. We use the SLMs, in addition, to correct the optical aberrations of the setup. The method we use to generate the phase masks is described in [1–3].

The three SLMs are arranged as sketched in Fig. A.1. The geometry of the trapping sites is sketched in Fig. A.2. All the trapping beams are generated from a 2 W laser of 821 nm wavelength (Toptica TA Pro). The three beams are overlapped with polarizing beamsplitter cubes and can be turned on or off independently using acousto-optic modulators (AOM, not shown in Fig. A.1).

- SLM1 prepares an array of  $13 \times 5 = 65$  Gaussian optical tweezers with a waist of  $1.2 \mu\text{m}$ , with an intersite spacing of  $6 \mu\text{m}$  and  $12.5 \mu\text{m}$  along the  $x$  and  $z$  axes, respectively. With a power of 2.6 mW per trapping site, the transverse and longitudinal trap oscillation frequencies are 80 kHz and 17 kHz, respectively;
- SLM2 prepares an array of four optical bottle beams (BoBs), separated by  $30 \mu\text{m}$  and  $25 \mu\text{m}$  along the  $x$  and  $z$  axes, respectively. The power per BoB is 22 mW, corresponding to transverse and longitudinal trap oscillation frequencies of 16 kHz and 5 kHz, respectively;
- SLM3 is either used to generate a single or an array of Gaussian optical tweezers. The shape of the optical tweezers is identical to that of those prepared by SLM1. This array of optical tweezers is meant to trap the ancilla atoms, while we use the single optical tweezer for the preparation of defect-free arrays of atoms. A

---

\* Corresponding author: clement.sayrin@lkb.ens.fr

telescope conjugates the plane of SLM3 with that of an acousto-optic deflector (AOD), so that a dynamically-controllable phase grating generated by the AOD is superimposed with the phase mask generated by SLM3. We use the AOD during an experimental sequence to either move a single (see sec. A 3) or an array (see sec. A 5) of Gaussian optical tweezers.

### 3. Preparation of the ensembles of trapped atoms

We initially load atoms into the array of optical tweezers prepared by SLM1, in the collisional blockade regime. We employ a 3D-MOT, initially loaded by a low-velocity atomic beam, originating from a 2D-MOT, that enters the vacuum chamber along the  $z$  axis. A subsequent optical-molasses stage cools the trapped atoms to  $13\mu\text{K}$ . A 25 ms-long fluorescence image, using the optical molasses beams, detects the trapped atoms. We measure an average loading probability per site of 62 %. We then use the single Gaussian optical tweezer generated by SLM3 to re-arrange the atoms into the target array [4], indicated in Fig. A.2.a by red circles. This array consists in four ensembles of either two or three atoms, depending on the number of ancillae per ensemble. We use a second fluorescence image to probe the effective preparation of a defect-free target array. All the data presented in this work are post-selected to keep only the experimental realizations for which the target array had no defects, and no additional atoms were left

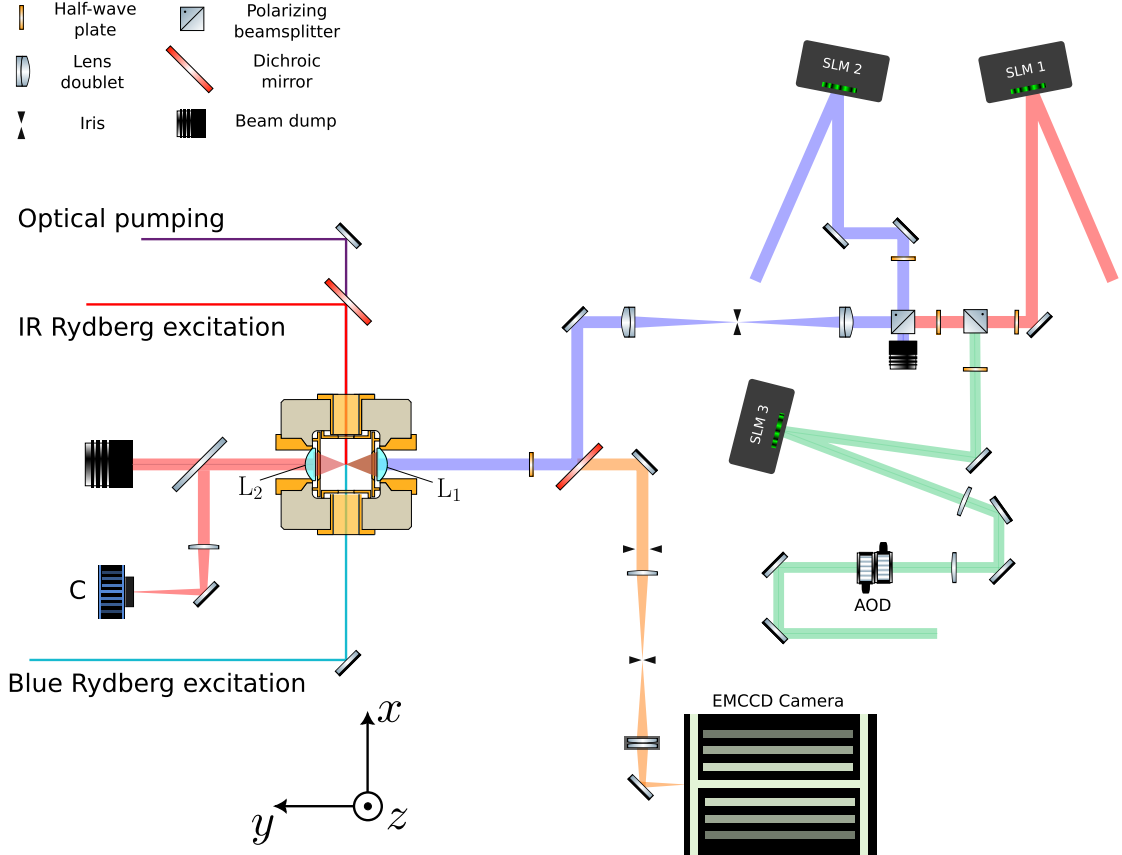

Figure A.1. **Sketch of the experimental setup.** A sapphire cube (beige, not to scale) holds two short-focal-length lenses (cyan) and electrodes (orange) that control the electric field. The blue and infra-red Rydberg excitation lasers (thin light blue and red lines) and the ground-state manipulation beam (thin violet line) enter the cube along the  $x$  axis. The three trapping light beams (red, violet and green) prepared by the three SLMs and overlapped with polarizing beamsplitter cubes enter the cube along the  $y$  axis and through lens  $L_1$ . The AOD is used to dynamically move the set of tweezers prepared by SLM3. A second lens  $L_2$  collects all trapping light, eventually focused on a monitoring camera (C). Fluorescence photons are collected by  $L_1$  and focused into the EMCCD camera. Several irises spatially filter the light to reduce stray light. The SLM planes are imaged onto lens  $L_1$  with a  $4f$  telescope with  $f = 400$  mm. An iris placed at the intermediate focal point of this telescope filters out non-diffracted light.

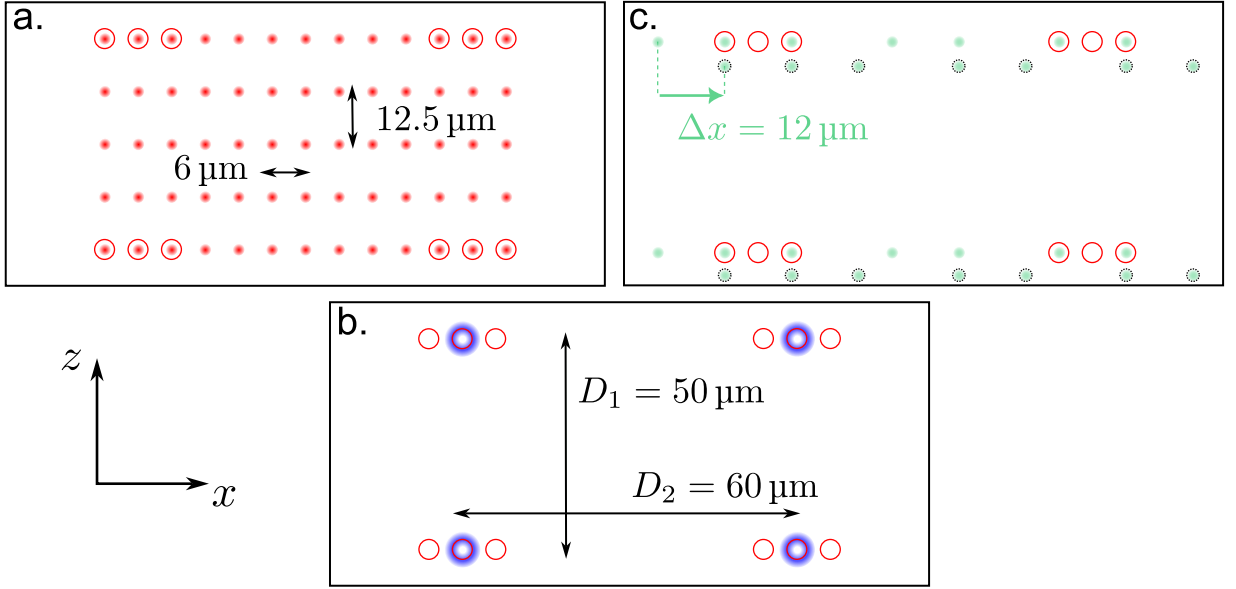

Figure A.2. **Geometries of the three arrays of trapping sites.** **a.** Arrays of Gaussian optical tweezers (red-gradient-filled circles) generated by SLM1. The 65 sites are arranged along a regular array with an intersite spacing of  $6\ \mu\text{m}$  and  $12.5\ \mu\text{m}$  along the  $x$  and  $z$  axes, respectively. The axis definition is identical to that of Fig. A.1. In all panels, the red open circles indicate the twelve sites of the target array, deterministically prepared with the re-arranger beam. For the experiments with one ancilla per ensemble, the right sites of the ensembles are left empty. **b.** Array of four optical bottle beams (violet rings), prepared by SLM2, that are used to trap the circular Rydberg atoms. **c.** Array of Gaussian optical tweezers (green-gradient-filled circles) prepared by SLM3, used to trap the ancilla atoms. The circles with dark dashed contour lines indicate the position of the trapping beams when the AOD shifts the whole array by  $\Delta x = 12\ \mu\text{m}$ . For clarity, they are shifted down along the  $z$  axis with respect to their actual positions. In this situation, there is no remaining light in two out of the eight original sites.

in the other trapping sites of SLM1.

After the second fluorescence image, we adiabatically lower the power of the trapping sites of SLM1 to  $0.16\ \text{mW}$ , cooling the atoms down to  $4.5\ \mu\text{K}$ . We increase the magnetic field to  $14\ \text{G}$  and optically pump all atoms to  $|1\rangle = |5S_{1/2}, F=2, m_F=3\rangle$  using a  $\sigma^+$  polarized laser beam on resonance with the  $|5S_{1/2}, F=2\rangle \rightarrow |5P_{3/2}, F'=2\rangle$  transition, in conjunction with a repumper laser beam on resonance with the  $|5S_{1/2}, F=1\rangle \rightarrow |5P_{3/2}, F'=2\rangle$  transition. Simultaneously, we change the phase mask applied on SLM3, so that it now prepares the array of trapping sites shown in Fig. A.2.c. We adiabatically turn on this array of trapping sites for the ancilla atoms up to  $1.0\ \text{mW}$  per site within  $0.5\ \text{ms}$ . At this stage, the atoms that will be used as ancillae are trapped in the superposition of two Gaussian optical tweezers, created by SLM1 and SLM3. Because of the large frequency difference ( $\approx 200\ \text{MHz}$ ) between the two laser beams and because of the significant intensity difference, however, the trapping potential is essentially controlled by the optical tweezers created by SLM3. The logical atoms are trapped in the low-power optical tweezers from SLM1 only.

#### 4. Experimental sequence

After the preparation stage described in the previous section, we run an experimental sequence, of which we sketch a typical example in Fig. A.3. The latter corresponds to the sequence of Fig. 4.c and the data of Fig. 4.d. At  $t = 0$ , we turn off the optical tweezers from SLM1, leaving the logical atoms untrapped. The ancillae are still trapped in the Gaussian tweezers of SLM3. The logical atoms are then excited to  $|52D_{5/2}, m_J = 5/2\rangle$  using a  $1\ \mu\text{s}$ -long two-photon optical  $\pi$  pulse with  $\sigma^+$  polarized laser beams of wavelengths  $420\ \text{nm}$  and  $1015\ \text{nm}$ , detuned by  $500\ \text{MHz}$  from the intermediate  $|6P_{3/2}, F'=3\rangle$  level. The ancillae are impervious to this excitation because of the  $8.6\ \text{MHz}$  trap-induced light shifts. We turn on the BoBs prepared by SLM2 right after the optical excitation.

A MW field at  $64.7566\ \text{GHz}$  transfers the logical atoms to  $|52F, m=2\rangle$ . We adiabatically increase the electric field to  $2.16\ \text{V} \cdot \text{cm}^{-1}$  while shining a  $\sigma^+$  polarized radiofrequency field at  $225\ \text{MHz}$  to transfer these atoms to the circular state  $|\downarrow\rangle = |52C\rangle$ . Then, we set the electric field to  $1.59\ \text{V} \cdot \text{cm}^{-1}$  to reach the required Förster resonance (see Sec. B) before running one of the sequences of MW and optical pulses described in the main text.

At the end of the sequence, all atoms in any ground state (including  $|0\rangle$  and  $|1\rangle$ ) are recaptured in the array of

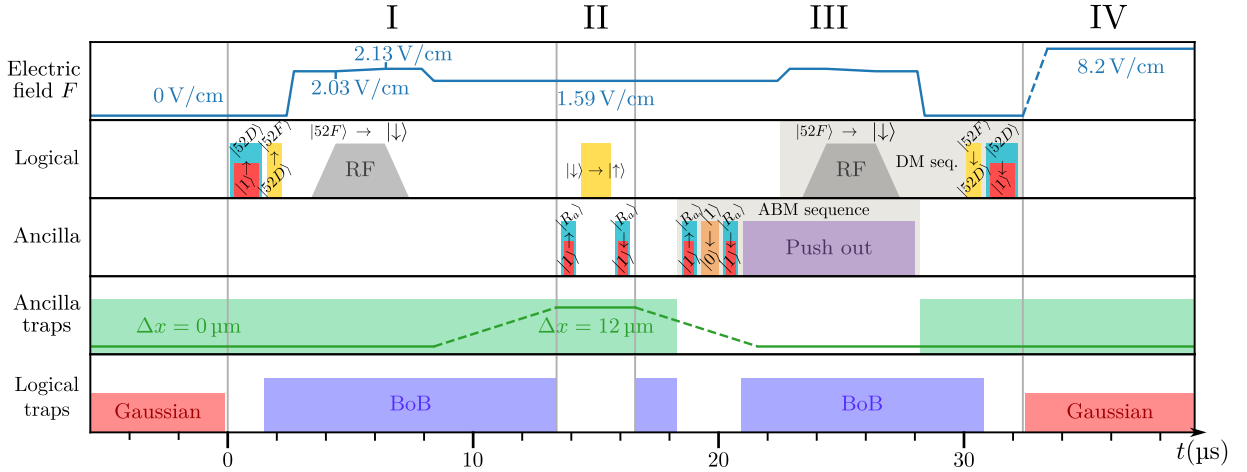

Figure A.3. **Typical experimental sequence run after the preparation of a defect-free array of individual atom**, which ends at  $t = 0$ . The sequence is schematically represented as a function of time. Its four main parts at  $t > 0$  correspond to (I) the preparation of the logical atom in  $|\downarrow\rangle$ , (II) local manipulation of the logical atom that corresponds to the data of Fig. 4.d, (III) the ABM and DM sequences used for the non-destructive and destructive measurement of the logical atom, and (IV) the final readout of the state with a fluorescence image (not shown) once the atoms have been recaptured in the optical tweezers of SLM1. Right after the last Rydberg excitation pulse, we increase the electric field to reduce the decay of residual Rydberg excitations to the ground state. First line: amplitude of the electric field. Second line: optical (blue and red), MW (yellow) and RF (grey) pulses applied to the logical atom. The trapeze form of the radiofrequency (RF) pulse corresponds to an adiabatic increase and reduction of the RF power. The transitions addressed by each pulse are superimposed with the color boxes. The decircularization process used for the DM is indicated by a light grey background. Third line: Same as the second line, but for the ancilla atoms. The orange and violet boxes correspond to the shelving and push-out stages, respectively, of the ABM sequence indicated by a light grey background. Fourth line: the green color box indicates when the trapping light from SLM3 is applied onto the ancilla atoms. The green line is a plot of the programmed shift of the whole array imposed by the AOD. The dashed line corresponds to the finite response time of the AOD during which the trapping array is changing. Fifth line: the red and blue boxes indicate when the trapping light from SLM1 (Gaussian) or SLM2 (BoB), respectively, is shone onto the atoms.

trapping sites prepared by SLM1. The two other arrays are turned off. We use a third fluorescence image, identical to the previous ones, to measure the probability to recapture the ancilla and logical atoms in their respective optical tweezers. To reduce the probability that an atom in a low- $\ell$  Rydberg state at the end of the sequence decays back to its ground-state and is detected by the final fluorescence image, we increase the electric field to  $8.2 \text{ V} \cdot \text{cm}^{-1}$  after the last optical pulse that transfers the  $|52D\rangle$  state back to  $|1\rangle$ . This strongly reduces the decay rates on optical transitions from Rydberg levels to the ground states, so that Rydberg atoms remain as long as possible in anti-trapped Rydberg levels and are expelled from the Gaussian optical tweezers well before the fluorescence imaging.

## 5. Manipulation of the ancillae

The optical excitation of the ancillae from  $|1\rangle$  to  $|R_a\rangle = |45S_{1/2}, m_J = 1/2\rangle$  is similar to that of the logical atoms. It employs the same 420 nm-wavelength light, together with a  $\sigma^-$  polarized 1017 nm-wavelength light, which is overlapped with the 1015 nm-wavelength beam used for the logical atoms. The optical  $\pi$  pulse that prepares  $|R_a\rangle$  lasts 0.4  $\mu\text{s}$ .

We turn off the BoBs during the optical excitation of the ancillae, from  $|1\rangle$  to  $|R_a\rangle$  or back, to avoid residual light-shifts. If all of the ancillae are to be excited, we turn off the laser beam impinging on SLM3 using an AOM (not shown in Fig. A.1). For the data of Fig. 4.d, however, only two out of eight ancillae should be excited to  $|R_a\rangle$ . To do this, using the AOD, we translate the array of trapping sites generated by SLM3 along the  $x$  axis by  $\Delta_x = 12 \mu\text{m}$ . Using the geometry shown in Fig. A.2, this translation effectively leaves only two ancillae untrapped, while the six other are still trapped after the displacement. The latter lasts 5  $\mu\text{s}$ , limited by the response time of the AOD. We find that we do not need to turn off the trapping light during the translation of the array to avoid atom losses.

The selective detection of state  $|1\rangle$  after step (ii) of the ABM sequence requires one to shelve state  $|1\rangle$  into  $|0\rangle$  [step (iii) of the ABM sequence]. We perform the shelving into  $|0\rangle$  with a 0.7  $\mu\text{s}$ -long pulse of optical pumping on the  $\pi$ -polarized  $|1\rangle \rightarrow |5P_{3/2}, F' = 2, m_F = 2\rangle$  transition. The corresponding laser beam enters the vacuum chamber with a  $45^\circ$  angle from the  $y$  and  $z$  axes (not shown in Fig. A.1) and has an intensity 170 times higher than the saturation

intensity of the transition. The atoms excited to  $|R_a\rangle$  at step (ii) are de-excited to  $|1\rangle$  at step (iv) of the ABM sequence and expelled from the traps at step (v), without affecting those in  $|0\rangle$ . We use a  $\sigma^+$  polarized push-out laser beam at resonance with the  $|1\rangle \rightarrow |5P_{3/2}, F' = 3, m_F = 3\rangle$ . Its intensity is 0.66 times the saturation intensity of the transition and we shine it during 7  $\mu$ s. It shares the same optical path as the laser used for the initial optical pumping into  $|1\rangle$ . During both the shelving and the push-out phases, we turn off the trapping laser beams of the ancillae.

## Appendix B: Stark-tuned Förster resonance

### 1. Choice of the Rydberg states

The QND measurement and the local manipulation of the logical atoms rely on the dipole blockade of optical or MW transitions in the presence of interactions between the logical atom in a circular Rydberg level  $|\uparrow\rangle = |nC\rangle$  and an ancilla in a laser-accessible low-angular-momentum ( $\ell$ ) Rydberg level  $|R_a\rangle$ . Strong first-order interactions between  $|\uparrow\rangle$  and  $|R_a\rangle$  require a Förster resonance. However, there is a priori no zero-field resonance for Rb between a pair of high- $\ell$  Rydberg levels  $|R_c\rangle, |nC\rangle$  and a couple of low- $\ell$  Rydberg states  $|R_a\rangle, |R'_a\rangle$ , with  $|R_a\rangle$  being laser accessible from the ground state and  $|R_a\rangle \rightarrow |R'_a\rangle$  and  $|R_c\rangle \rightarrow |nC\rangle$  being electric-dipole-allowed transitions. Therefore, we rather rely on a Stark-tuned Förster resonance [5, 6]: we seek pair states  $|R_a, R'_a\rangle$  and  $|nC, R_c\rangle$  at resonance in an experimentally-convenient electric field of a few  $\text{V} \cdot \text{cm}^{-1}$ .

In order to maximize the strength of the interaction, the electric dipole matrix elements of the  $|R_a\rangle \rightarrow |R'_a\rangle$  and  $|R_c\rangle \rightarrow |nC\rangle$  transitions should be as large as possible, leading to the choice of  $|R_c\rangle = |(n \pm 1)C\rangle$ . In addition, we restrict ourselves to the situation where the electric field is parallel to the interatomic axis. The conservation of angular momentum then imposes the polarization of the  $|R_a\rangle \rightarrow |R'_a\rangle$  to match that of the  $|(n \pm 1)\rangle \rightarrow |nC\rangle$  transition, i.e., to be  $\sigma^+$ . In Fig. B.1.a, we represent as a function of  $n$  and of the resonance electric field,  $F_{\text{res}}$ , all Förster resonances we have found between a circular-Rydberg-level pair state  $|nC, (n+1)C\rangle$ ,  $43 \leq n \leq 70$ , and a low- $\ell$  Rydberg pair state  $|R_a, R'_a\rangle$ , where  $|R_a\rangle$  and  $|R'_a\rangle$  are  $S$ ,  $P$  or  $D$  states, and for which  $|R_a\rangle \rightarrow |R'_a\rangle$  is  $\sigma^+$  polarized. The colour code indicates the strength of the dipole matrix element of the  $|R_a\rangle \rightarrow |R'_a\rangle$  transition. When different pair states differ only through the quantum numbers  $m$  or  $m_J$ , we plot only the pair states with the maximum  $m$  value, i.e., with the largest dipole.

In our setup, because of MW and RF bandwidth limitations, we cannot efficiently manipulate circular states with  $n \gtrsim 55$ . We also prefer to work at low field values to reduce the decoherence induced by electric field noise, though high enough to preserve the stability of circular states. This led us to choose the states  $|R_c\rangle = |53C\rangle$ ,  $|R_a\rangle = |45S_{1/2}, m_J = +1/2\rangle \equiv |45S\rangle$  and  $|R'_a\rangle = |45P_{3/2}, m_J = +3/2\rangle \equiv |45P\rangle$ . The pair states  $|53C, 45P\rangle$  and  $|54C, 45S\rangle$  are on resonance in a field of  $F_{\text{res}} = 1.598 \text{ V/cm}$ . The resonant spin-exchange-interaction rate between these levels is  $\Omega = 2V/h = 21 \text{ MHz}$ , when the logical and ancilla atoms are  $6.0 \mu\text{m}$  away.

### 2. Förster resonance spectroscopy

We probe the Förster resonance between the ancilla and logical atoms by measuring, for different values of the applied electric field, the laser excitation spectrum of the  $|1\rangle \rightarrow |R_a\rangle = |45S_{1/2}, m_J = +1/2\rangle$  transition, when the logical atom is prepared in  $|\uparrow\rangle = |54C\rangle$ . The experimental sequence is similar to that used for the data shown in Fig. 2.b of the main text, but the Rydberg-excitation optical pulse lasts here 0.3  $\mu$ s. The spectrum shown on Fig. B.1.b is measured close to the Förster resonance. It shows three peaks because, in contrast to the data of Fig. 2 of the main text, we do not post-select the data on the destructive measurement of the logical atom in  $|54C\rangle$ . Thus, the middle peak, which corresponds the excitation of  $|45S\rangle$  for an isolated ancilla atom, results from a failed preparation of  $|54C\rangle$  for the logical atom. The top and bottom peaks correspond to the excitation of the interaction eigenstates, which read

$$|\pm\rangle_{\Delta_p} = \cos(\theta) |54C, 45S\rangle \pm \sin(\theta) |53C, 45P\rangle . \quad (\text{B1})$$

In Eq. (B1),  $\tan(2\theta) = \Omega/\Delta_p$ , with  $h\Delta_p$  the electric-field dependent energy difference between  $|53C, 45P\rangle$  and  $|54C, 45S\rangle$ . The frequency difference  $\Delta_p$  can be expressed as a function of the electric field, through the differential Stark effect coefficients,  $\alpha_{SP}^{(1)} = -3.667 \text{ MHz/(V/cm)}$ ,  $\alpha_{SP}^{(2)} = -55.568 \text{ MHz/(V/cm)}^2$  and  $\alpha_{CC}^{(2)} = -0.339 \text{ MHz/(V/cm)}^2$ , between  $|45S\rangle$  and  $|45P\rangle$  and between  $|53C\rangle$  and  $|54C\rangle$ , respectively:

$$\Delta_p = \alpha_{SP}^{(1)} (F - F_{\text{res}}) + \left( \alpha_{SP}^{(2)} - \alpha_{CC}^{(2)} \right) (F^2 - F_{\text{res}}^2) . \quad (\text{B2})$$

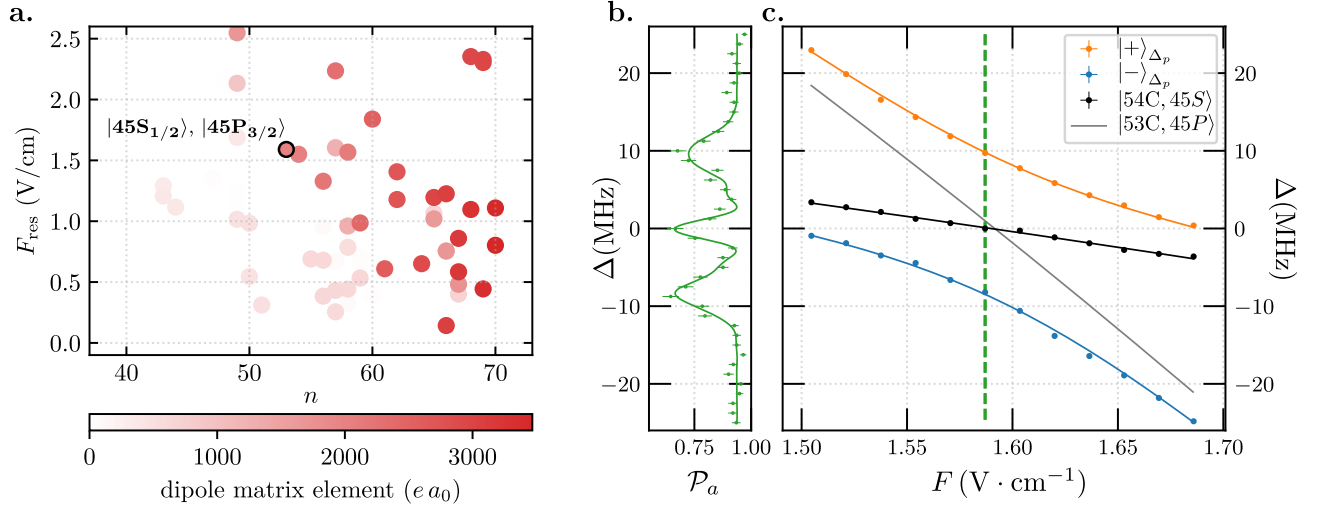

Figure B.1. **Choice and spectral evidence of a Förster resonance.** **a.** Map of the low-angular-momentum Rydberg pair states  $|R_a, R'_a\rangle$  that have a Stark-tuned Förster resonance with a circular-Rydberg pair states  $|nC, (n+1)C\rangle$ . Each point corresponds to a resonance, plotted as a function of  $n$  and the resonance electric field  $F_{\text{res}}$ . The colour scale gives the dipole matrix element of the  $|R_a\rangle \rightarrow |R'_a\rangle$  transition in units of  $(ea_0)$ . The pair state used for our experiments is highlighted by a dark circle. **b.** Probability  $\mathcal{P}_A$  to recapture an ancilla atom excited to  $|45S_{1/2}, m_J = 1/2\rangle$  in the vicinity of a logical atom prepared in  $|54C\rangle$  in an electric field of  $F = 1.591 \text{ V} \cdot \text{cm}^{-1}$ . The experimental sequence is similar to that used for the data of Fig. 2 of the main text. The green solid line is a fit to the data of a sum of two Gaussian peaks and of a coherent-excitation profile (B4). **c.** Fitted resonant frequencies of the three peaks observed in the excitation spectrum of panel **b** plotted as a function of  $F$ . Orange, blue and black data points correspond to the highest, lowest and central measured frequencies. They correspond to the frequencies of the transitions from  $|54C, 5S\rangle$  to  $|+\rangle_{\Delta_p}$  (orange points),  $|-\rangle_{\Delta_p}$  (blue points) with interacting atoms, or to  $|54C, 45S\rangle$  (black points) for non-interacting atoms. The black line is a fit of Eq. (B5) to the black data points, the orange and blue lines are fits of Eq. (B6) to the orange and blue data points. The light grey line indicates the energy difference between the non-interacting pair states  $|54C, 5S\rangle$  and  $|53C, 45P\rangle$ . An anti-crossing, signature of the Förster resonance between the ancilla and logical atoms, is apparent. The green dashed line indicates the electric field used in the experiments of the main text.

The energies of  $|\pm\rangle_{\Delta_p}$  read

$$E_{\pm} = \frac{\hbar\Delta_p}{2} \pm \frac{\hbar}{2} \sqrt{\Omega^2 + \Delta_p^2}. \quad (\text{B3})$$

We analyze the spectra plotted in Fig. 2.b of the main text and in Fig. B.1 in a similar way. The central peak is well fitted by a coherent excitation profile that takes the form of

$$\mathcal{P}(\Delta) = \mathcal{P}_0 + A \frac{\Omega^2}{\Omega^2 + \Delta^2} \sin^2\left(\pi \sqrt{\Omega^2 + \Delta^2} T\right), \quad (\text{B4})$$

where  $\Omega$  is the Rabi frequency of the optical excitation,  $T = 0.4 \mu\text{s}$  (Fig. 2) or  $0.3 \mu\text{s}$  (Fig. B.1) the duration of the pulse, and the coefficients  $\mathcal{P}_0$  and  $A$  account for a  $\Delta$ -independent limited recapture efficiency of the ancillae and a limited efficiency of the Rydberg excitation, respectively. For the data of Fig. 2, we find  $\Omega = 1.30(5) \text{ MHz}$ ,  $\mathcal{P}_0 = 0.997(5)$ ,  $A = 0.99(1)$ . The full width at half maximum (FWHM) for this peak is  $2.08(8) \text{ MHz}$ .

The two outer peaks, however, are broadened by the thermal spread of the positions of the ancilla and logical atoms in their traps. Thus, we rather fit Gaussian profiles to these two peaks, and find, for the data of Fig. 2, a FWHM of  $4.0(2) \text{ MHz}$  for the right peak and  $3.8(1) \text{ MHz}$  for the left peak. The measured broadening with respect to the central peak is compatible with a thermal spread of the atoms with a temperature of  $T = 4.5 \mu\text{K}$  and a trap oscillation frequency of  $20 \text{ kHz}$ .

We plot in Fig. B.1.c the frequencies of the three observed peaks as a function of  $F$ , obtained by fitting to the data of Fig. B.1.b a sum of two Gaussian peaks and of a coherent excitation profile (B4). The frequency of the central peak depends on  $F$  through the Stark effect of  $|45S\rangle$  only, and can be expressed as  $\nu_{\text{res}} + \Delta_0(F)$ , where  $\nu_{\text{res}}$  is the frequency of the  $|1\rangle \rightarrow |45S\rangle$  transition when  $F = F_{\text{res}}$  or, similarly, of the  $|54C, 5S\rangle \rightarrow |54C, 45S\rangle$  transition without dipole-dipole interaction. The frequency difference  $\Delta_0(F)$  reads

$$\Delta_0(F) = \alpha_{45S}^{(1)} (F - F_{\text{res}}) + \alpha_{45S}^{(2)} (F^2 - F_{\text{res}}^2), \quad (\text{B5})$$

where  $\alpha_{45S}^{(2)} = 0.537 \text{ MHz}/(\text{V}/\text{cm})^2$  and  $\alpha_{45S}^{(1)} = -12.322 \text{ MHz}/(\text{V}/\text{cm})$  are the quadratic and linear Stark coefficients of  $|45S\rangle$  calculated for a field  $F \approx 1.6 \text{ V} \cdot \text{cm}^{-1}$  [7]. The electric-field-dependent frequencies of the  $|54C, 5S\rangle \rightarrow |\pm\rangle_{\Delta_p}$  transitions, corresponding to the two outer peaks, read  $\nu_{\text{res}} + \Delta_{\pm}(F)$ , with

$$\Delta_{\pm}(F) = \Delta_0(F) + \frac{1}{2}\Delta_p(F) + \frac{E_{\pm}(F)}{2} = \Delta_0(F) + \frac{1}{2}\Delta_p(F) \pm \frac{1}{2}\sqrt{\Omega^2 + \Delta_p(F)^2}. \quad (\text{B6})$$

We fit Eq. (B5) and (B6) to the data of Fig. B.1.c with  $\Omega$ ,  $F_{\text{res}}$  and  $\nu_{\text{res}}$  as free parameters. We find  $F_{\text{res}} = 1.592(1) \text{ V}/\text{cm}$  and  $\Omega = 18.2(1) \text{ MHz}$ , which corresponds to an inter-atomic distance of  $6.27(2) \mu\text{m}$ . The discrepancy with the measured  $6.1 \mu\text{m}$  distance with the data of Fig. 2 can be explained by the fact that the phase masks used for the two experiments, performed a couple months apart, are slightly different.

## Appendix C: Estimation of the ABM fidelities

### 1. Procedure

In this section, we describe the model used to obtain a precise estimation of the non-destructive measurement efficiencies,  $\eta_{\uparrow}$  and  $\eta_{\downarrow}$ , defined as the probability to block the optical excitation of the ancilla to  $|R_a\rangle$  when the logical atom is in  $|\uparrow\rangle$  and the probability to excite the ancilla to  $|R_a\rangle$  when the logical atom is in  $|\downarrow\rangle$ . The measured spectra of Fig. 2 of the main text and the values of  $\mathcal{P}_A$  at resonance would be sufficient to estimate  $\eta_{\uparrow}$  and  $\eta_{\downarrow}$ , would the DM be error free. For a proper estimation of the ABM efficiency, we need to consider the limitations of the DM scheme. The latter are, e.g., responsible for the small peak around  $\Delta = 0$ , in the data of Fig. 2.b, when the logical atom has been measured by the DM scheme in  $|\uparrow\rangle$  (see main text).

To do so, we repeat the experiments presented in Fig. 3.a of the main text, with and without the MW  $\pi$  pulse that transfers  $|\uparrow\rangle$  to  $|\downarrow\rangle$  after the ABM sequence; the destructive measurement effectively measures the probability to have the logical atom in  $|\uparrow\rangle$  and  $|\downarrow\rangle$ , respectively. In Fig. C.1.b and c, we plot the joint probabilities to detect the logical and ancilla atoms without and with the final MW  $\pi$  pulse. The possible outcomes are labelled with the following terminology: Filled and open symbols indicate an atom eventually detected and absent, respectively, in the final fluorescence image. The left triangles ( $\blacktriangleright$ ,  $\triangleright$ ) correspond to the ancilla to the left of the logical atom in Fig. A.2, the right triangles ( $\blacktriangleleft$ ,  $\triangleleft$ ) to the right ancilla, and the central circles ( $\bullet$ ,  $\circ$ ) to the logical atom. The large circle ( $\bigcirc$ ) is specifically used to represent a logical atom in  $|\uparrow\rangle$ . A  $\times$  in place of the previously defined symbols corresponds to any possible state.

Every triplet of symbols denotes the conjoined presence or absence of the three atoms. When present, an index indicates the index (1, 2 or 3) of the fluorescence image used to measure the probability of the considered event. The starting event  $\blacktriangleright_2 \bullet_2 \blacktriangleleft_2$  correspond to the three atoms present in the second fluorescence image, made after the rearrangement of the initially loaded array. The notation  $\mathbb{P}_2(X)$  corresponds to the probability of event  $X$  conditioned on the effective realization of  $\blacktriangleright_2 \bullet_2 \blacktriangleleft_2$ , namely of the preparation of the defect-free target array.

In the model we develop, the two ancillae are perfectly symmetric: the model does not distinguish the  $\triangleright \times \blacktriangleleft$  and  $\blacktriangleright \times \triangleleft$  events. Therefore, for these asymmetrical events, we calculate instead the sum of their probabilities, leaving only 5 independent triplet of events:  $\blacktriangleright \bullet \blacktriangleleft$ ,  $\blacktriangleright \circ \blacktriangleleft$ ,  $\triangleright \bullet \triangleleft$ ,  $\triangleright \circ \triangleleft$ ,  $(\blacktriangleright \bullet \blacktriangleleft) \cup (\blacktriangleleft \bullet \triangleright)$ . We deduce the probability of the remaining event  $(\triangleright \circ \blacktriangleleft) \cup (\blacktriangleleft \circ \triangleright)$  from the five others. We measure these five independent probabilities at the end of the experimental sequence and plot them in Fig. C.1.b and c as a function of the MW pulse duration,  $\tau$ .

### 2. Details of the model

In order to understand the contrast of the oscillations observed in Fig. C.1, we develop a model summarized in the form of a probability tree sketched on Fig. C.1.a. It includes 13 independent parameters, listed below:

- $\eta_{\uparrow}$ , measurement efficiency of  $|\uparrow\rangle$ ;
- $\eta_{\downarrow}$ , measurement efficiency of  $|\downarrow\rangle$ ;
- $p_{\text{circ.}}$ , the circularization efficiency, namely the probability for an atom in  $|52F\rangle$  to be transferred to  $|52C\rangle$  with the first RF adiabatic passage;
- $p_{\text{decirc.}}$ , the de-circularization efficiency, namely the probability for an atom in  $|52C\rangle$  to be transferred to  $|52F\rangle$  with the second RF adiabatic passage;
- $p_{52F}$ , the probability that the logical atom remains in  $|52F\rangle$  after the circularization process. It differs from  $1 - p_{\text{circ.}}$  because the atom may be left by the circularization process in a state different from  $|52F\rangle$  or  $|52C\rangle$ . In the following, we denote  $|52X\rangle$  any state other than  $|52F\rangle$ ,  $|52C\rangle$  and  $|54C\rangle$ ;

a.

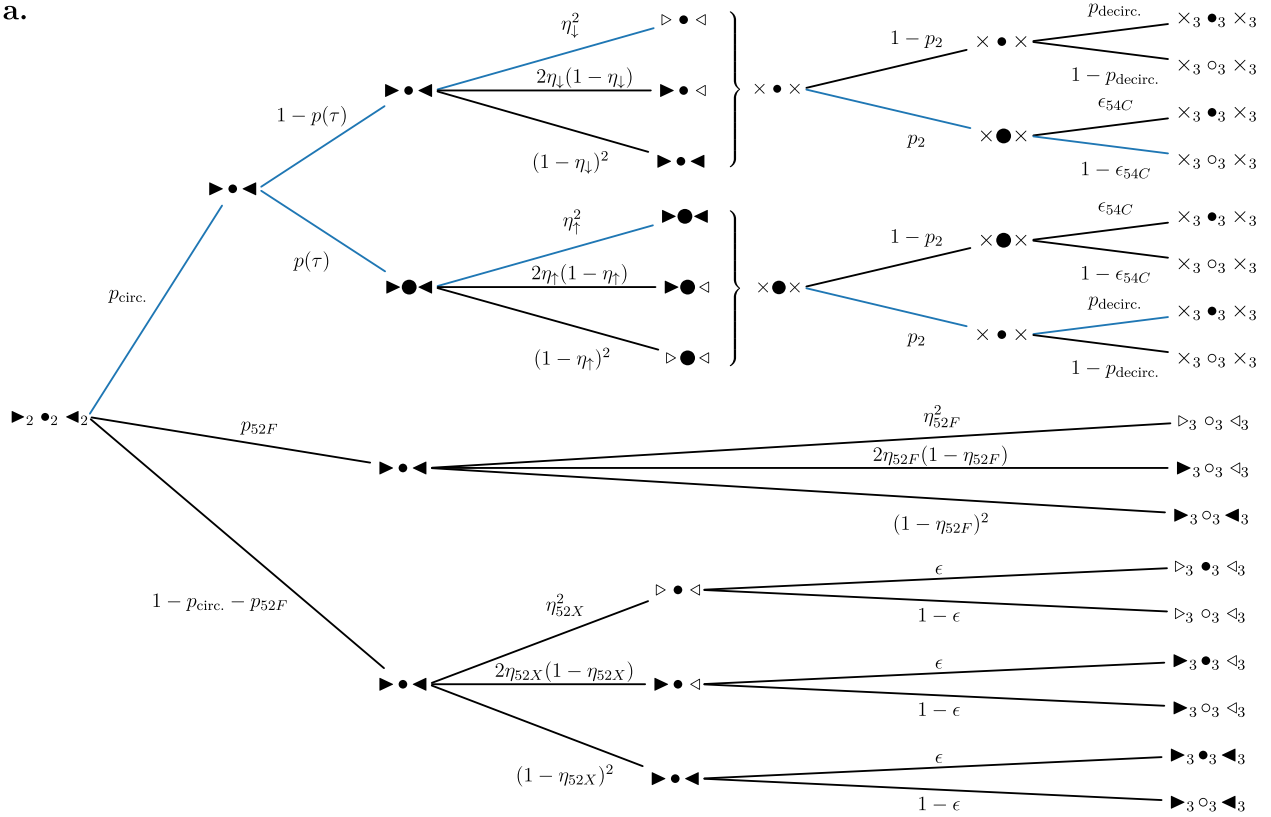

b.

|52C&gt;-state destructive measurement

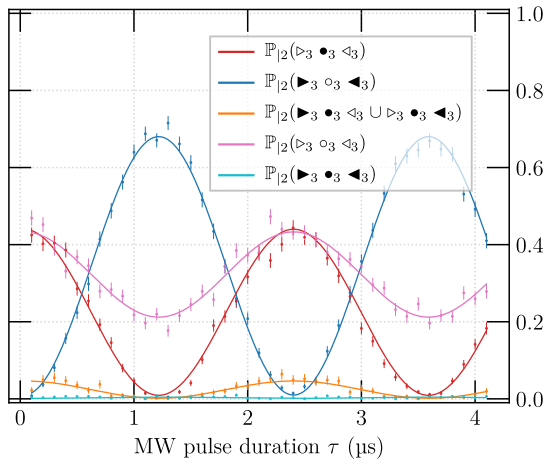

**C.**

|54C&gt;-state destructive measurement

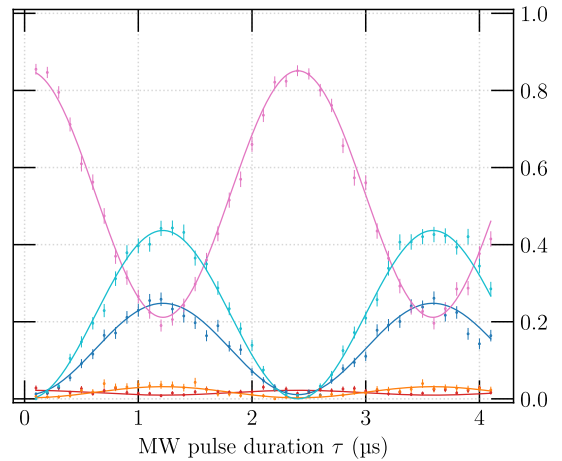

Figure C.1. **Error model and fit to the data.** **a.** Probability tree corresponding to the measurements of Rabi oscillations with the ABM and the DM. The tree is drawn in the situation of Fig. 3.a and b of the main text, namely when a MW  $\pi$  pulse is used after the ABM sequence to measure the state  $|\uparrow\rangle = |54C\rangle$  with the DM. The blue branches represent the two error-free paths. The symbol  $\times$  is used for compactness: it denotes any of the ancilla symbols ( $\blacktriangleright, \triangleright, \blacktriangleleft, \triangleleft$ ) of a previous branch. The branches drawn after the curly brackets are meant to be reproduced three times with the three considered configurations of ancillae. For the events with different outcomes for the two ancillae, we draw only one configuration to account for the two possible symmetric ones. **b., c.** Measured conditional probabilities of the five relevant events without (b.) and with (c.) the final MW  $\pi$  pulse that transfers atom in  $|\uparrow\rangle$  to  $|\downarrow\rangle$  before the DM scheme. In the two panels, the points are measurement outcomes, with the colour code given in the inset of panel b. The solid lines are the model curves fitted to the data with the parameters of Tab. I.



- $p_1$ , the efficiency of the first MW pulse that transfers  $|52C\rangle$  to  $|54C\rangle$ . More precisely, the transfer probability reads, as a function of the variable duration  $\tau$  of the MW pulse,  $p(\tau) = p_1 \sin^2[\frac{\pi}{2}(\tau - \delta\tau)/\tau_\pi]$ ;
- $\tau_\pi$ , the duration of the aforementioned  $\pi$  pulse;
- $\delta\tau$ , a phase parameter used to account phenomenologically for imperfect square pulses;
- $p_2$ , the efficiency of the second fixed-duration MW  $\pi$  pulse that follows the ABM sequence, used only for the data of Fig. C.1.c;
- $\epsilon_{54C}$ , the probability that the de-circularization process transfers an atom in  $|54C\rangle$  to a low- $\ell$  state that eventually decays to the ground state and is recaptured in the Gaussian tweezers at the end of the sequence;
- $\eta_{52F}$ , the probability to excite an ancilla atom to  $|R_a\rangle$  when the logical atom is in  $|52F\rangle$ . It accounts for the fact that the static electric dipole of  $|52F\rangle$  in  $F_{\text{res}}$  is strong enough to shift the excitation line of the ancilla to  $|R_a\rangle$  by 0.86(4) MHz and, therefore, to partially block the excitation;
- $\eta_{52X}$ , the probability to excite an ancilla atom to  $|R_a\rangle$  when the logical atom is in a state  $|52X\rangle$ ;
- $\epsilon$ , the probability to recapture in the Gaussian tweezers at the end of the sequence the logical atom in a state  $|52X\rangle$ .

The probabilities  $p_{52F} = 3.9\%$  and  $\eta_{52F} = 46\%$  have been measured independently with dedicated experiments. The 11 other parameters are free parameters of the model. Note that we single out the state  $|52F\rangle$ , and do not include it in the  $|52X\rangle$  states, for two reasons. On the one hand,  $|52F\rangle$  can partially block the excitation of the ancilla to  $|R_a\rangle$ , contrarily to, e.g.,  $|52D\rangle$ ,  $|53C\rangle$  or other high- $\ell$  Rydberg levels. On the other hand, if the logical atom is in  $|52F\rangle$  during the ABM sequence, there is a high chance that it will be transferred to  $|52C\rangle$  by the second RF adiabatic passage. For simplicity, we consider that those atoms cannot be eventually recaptured. Other Rydberg levels, included in  $|52X\rangle$ , may have a non-negligible probability to be recaptured, accounted for by the average coefficient,  $\epsilon$ .

### 3. Fit results

Using the probability tree, we calculate as a function of  $\tau$  and of the parameters defined above the probabilities of the 5 events plotted in Fig. C.1, in the two realizations of subfigures b and c. The 10 probabilities are sinusoidal functions of  $\tau$  with common period  $\tau_\pi$  and phase  $\delta\tau$ . We express their 10 contrasts and mean values as a function of the 9 other free parameters,  $p_{52F}$  and  $\eta_{52F}$ . We plot the fitted curves in Fig. C.1.b and c as solid lines. We find a good agreement with the experiment for the values of the parameters given in Tab. I.

| Parameters           | Fitted value           |
|----------------------|------------------------|
| $p_{\text{circ.}}$   | 72.3(4) %              |
| $\epsilon_{54C}$     | 0.7(1) %               |
| $p_{\text{decirc.}}$ | 66.0(4) %              |
| $\epsilon$           | 4.4(4) %               |
| $\eta_\uparrow$      | 96.6(2) %              |
| $p_1$                | 100 %                  |
| $\eta_\downarrow$    | 95.0(3) %              |
| $p_2$                | 97.9(4) %              |
| $\eta_{52X}$         | 93.7(9) %              |
| $\delta\tau_p$       | 0.06(1) $\mu\text{s}$  |
| $\tau_\pi$           | 1.187(3) $\mu\text{s}$ |
| Parameters           | Measured value         |
| $p_{52F}$            | 3.7(4) %               |
| $\eta_{52F}$         | 46(2) %                |

Table I. Fitted values of the 11 free parameters of the model and of  $p_{52F}$  and  $\eta_{52F}$  estimated with independent measurements. The fitted probabilities are bounded to the  $[0, 1]$  interval.

### 4. Imperfections analysis

In this section, we identify the main imperfections that limit the fitted values of  $\eta_\uparrow$  and  $\eta_\downarrow$ . Table II sums up these different imperfections and provides estimates of their contributions to the measurement efficiencies. These contributions have been calculated or measured independently via auxiliary experiments. They have not been included in the model to avoid significant complication of the probability tree.

The measurement efficiency,  $\eta_{\uparrow}$ , of  $|54C\rangle$  is limited by losses of an ancilla atom, when it should have been shelved in  $|0\rangle$  during the ABM sequence and eventually detected in the final fluorescence image. The first loss source stems from collisions with the background gas, and is estimated to 1.5 % over the  $\sim 84$  ms delay time between the second and third fluorescence images of the experimental sequence, given the 5.8 s lifetime of atoms in the traps. The second loss source originates from photoionization of the ancillae during the excitation of the logical atom to  $|52D\rangle$ . Photoionization is induced by the 420 nm-wavelength blue laser in presence of the 821 nm-wavelength 1 mW-power trapping light. Additional losses are induced by the fluorescence imaging itself and the optical pumping stage (0.5 %) Remarkably, these imperfections suffice to explain the value of  $\eta_{\uparrow}$ . In particular, we find no limitations due to an eventual imperfect dipole blockade of the excitation of the ancillae to  $|R_a\rangle$ .

The measurement efficiency,  $\eta_{\downarrow}$ , of the state  $|52C\rangle$  is limited by four main imperfections, that lead to a final recapture of the ancilla atom even though it should have been excited to  $|R_a\rangle$  and eventually expelled from the traps. The first one is the 51  $\mu$ s lifetime of  $|R_a\rangle = |45S_{1/2}, m_J = +1/2\rangle$ . An ancilla in  $|R_a\rangle$  can decay back to  $|0\rangle = |5S_{1/2}, F = 1\rangle$  prior to the second Rydberg excitation pulse that transfers  $|R_a\rangle$  back to  $|1\rangle$ . The second limitation corresponds to an imperfect excitation of  $|1\rangle$  to  $|R_a\rangle$ , which may stem from laser phase noise. The excitation efficiency is also limited by a limited preparation efficiency of  $|1\rangle$ . In particular, the 1.0 mW optical tweezers that trap the ancillae can pump the atoms out of the  $|1\rangle$  state over the 6 ms before the Rydberg excitation of the ancillae. The finite efficiency of the initial optical pumping itself to  $|1\rangle$  constitutes the fourth considered imperfection.

| 54C>-state measurement     |            | 52C>-state measurement     |            |
|----------------------------|------------|----------------------------|------------|
| Imperfection               | Estimation | Imperfection               | Estimation |
| Collisions                 | 1.5 %      | Lifetime                   | 1.3 %      |
| Photoionization            | 1.4 %      |                            |            |
| Imaging and pumping        | 0.5 %      | Phase noise                | 0.9 %      |
|                            |            | Trap de-pumping            | 0.5 %      |
|                            |            | Optical pumping            | 0.4 %      |
| Total                      | 3.4 %      | Total                      | 4.1 %      |
| Measured: $1 - \eta_{54C}$ | 3.4(2) %   | Measured: $1 - \eta_{52C}$ | 5.0(3) %   |

Table II. Experiment imperfections limiting the QND measurement efficiencies.

- 
- [1] B. Ravon, P. Méhaignerie, Y. Machu, A. D. Hernández, M. Favier, J. M. Raimond, M. Brune, and C. Sayrin, Array of Individual Circular Rydberg Atoms Trapped in Optical Tweezers, *Physical Review Letters* **131**, 093401 (2023).
  - [2] Y. Machu, C. Sayrin, and M. Brune, Patent FR 3 157 944, *Procédé de Génération Holographique d'un Réseau de Points de Focalisation* (2023).
  - [3] Y. Machu *et al.*, in preparation. (2025).
  - [4] D. Barredo, S. de Léséleuc, V. Lienhard, T. Lahaye, and A. Browaeys, An atom-by-atom assembler of defect-free arbitrary two-dimensional atomic arrays, *Science* **354**, 1021 (2016).
  - [5] G. Günter, H. Schempp, M. Robert-de-Saint-Vincent, V. Gavryusev, S. Helmrich, C. S. Hofmann, S. Whitlock, and M. Weidemüller, Observing the Dynamics of Dipole-Mediated Energy Transport by Interaction-Enhanced Imaging, *Science* **342**, 954 (2013).
  - [6] S. Ravets, H. Labuhn, D. Barredo, L. Beguin, T. Lahaye, and A. Browaeys, Coherent dipole-dipole coupling between two single Rydberg atoms at an electrically-tuned Forster resonance, *Nat Phys* **10**, 914 (2014).
  - [7] S. Weber, C. Tresp, H. Menke, A. Urvoy, O. Firstenberg, H. P. Büchler, and S. Hofferberth, Calculation of Rydberg interaction potentials, *Journal of Physics B: Atomic, Molecular and Optical Physics* **50**, 133001 (2017).
